# Supplementary material for: Traps and transport resistance: the next frontier for stable state-of-the-art non-fullerene acceptor solar cells
Source: arXiv:2203.11905 source file (2022-03-22)
Supplement: Supplementary file 1 [file SI.pdf]

# Supplementary Information for Traps and transport resistance: the next frontier for stable state-of-the-art non-fullerene acceptor solar cells

Christopher Wöpke,[1] Clemens Göhler,[1] Maria Saladina,[1] Xiaoyan Du,[2,3] Li Nian,[2,4] Christopher Greve,[5] Chenhui Zhu,[6] Kaila M. Yallum,[7] Yvonne J. Hofstetter,[8] David Becker-Koch,[8] Ning Li,[2,3] Thomas Heumüller,[2,3] Ilya Milekhin,[1] Dietrich R. T. Zahn,[1] Christoph J. Brabec,[2,3] Natalie Banerji,[7] Yana Vaynzof,[8] Eva M. Herzig,[5] Roderick C.I. MacKenzie,[9] and Carsten Deibel[1]

[1]*Institut für Physik, Technische Universität Chemnitz, 09126 Chemnitz, Germany*
[2]*Institute of Materials for Electronics and Energy Technology (i-MEET), Friedrich-Alexander-Universität Erlangen-Nürnberg, 91054 Erlangen, Germany*
[3]*Helmholtz Institute Erlangen-Nürnberg for Renewable Energy (HI ERN), Immerwahrstrasse 2, 91058 Erlangen, Germany*
[4]*Guangdong Provincial Key Laboratory of Optical Information Materials and Technology, Institute of Electronic Paper Displays, South China Academy of Advanced Optoelectronics, South China Normal University, Guangzhou, 510006 P. R. China*
[5]*Physikalisches Institut, Dynamik und Strukturbildung - Herzig Group, Universität Bayreuth, Universitätsstr. 30, 95447 Bayreuth, Germany*
[6]*Advanced Light Source, Lawrence Berkeley National Laboratory, Berkeley, California 94720, United States*
[7]*Department of Chemistry and Biochemistry, University of Bern, 3012 Bern, Switzerland*
[8]*Integrated Center for Applied Photophysics and Photonic Materials and the Center for Advancing Electronics Dresden, Technische Universität Dresden, 01062 Dresden, Germany*
[9]*Faculty of Engineering, University of Nottingham, Nottingham, Nottinghamshire NG7 2RD, United Kingdom*

## CONTENTS

# I. VARIABLE ANGLE SPECTROSCOPY ELLIPSOMETRY (VASE)

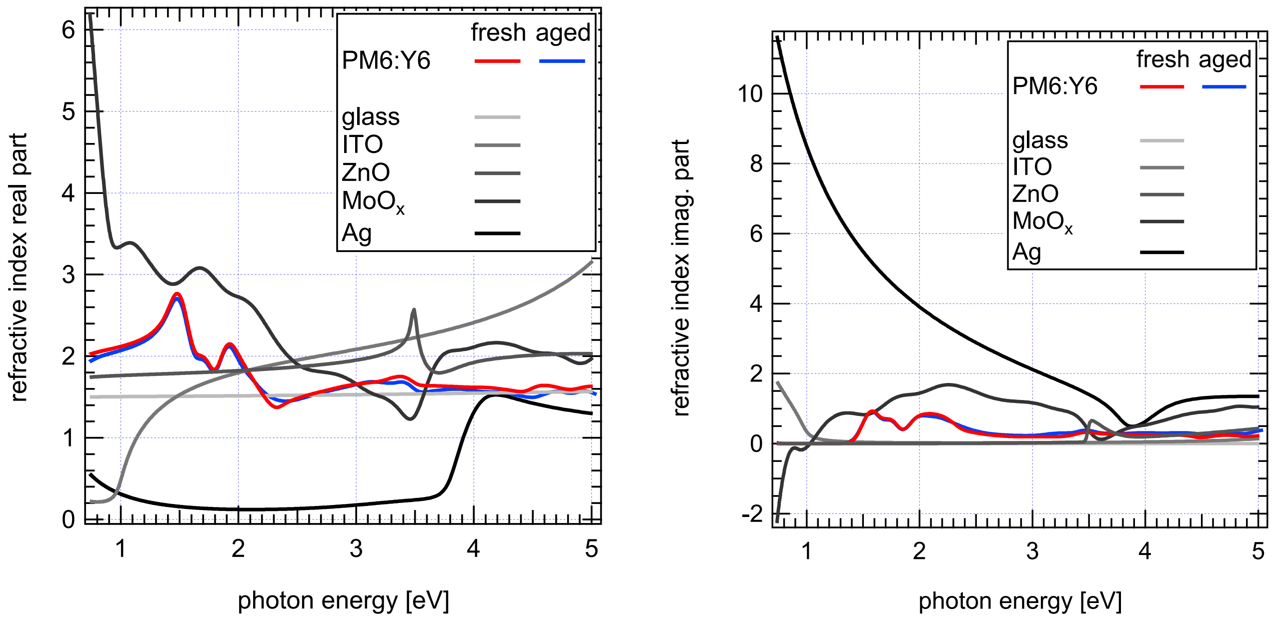


FIG. 1. Optical constants $n$ and $k$ measured with VASE for every layer of the solar cell stack as well as for a complete device, fresh and aged.

At first, the layer thickness of ITO and ZnO was determined from the spectra recorded on the ITO/ZnO bilayer structure on the glass substrate. The optical constants of the glass, ITO, and ZnO were used from Woollam's CompleteEASE database and the thickness of ITO and ZnO were the fit parameters. Once a reasonable fit of experimental data and optical model was obtained (multi-sample analysis, MSA), the optical constants of ITO and ZnO were tuned to best fit the experimental data. The optical constants and the thickness of ITO and ZnO were kept fixed in the proceeding samples.

After three samples with the varying thickness of PM6:Y6 mixture deposited on glass substrate/ITO/ZnO. The spectra from these samples were modeled using the MSA method. For this, the optical constants of the PM6:Y6 mixture were the common fit parameters, whereas the thickness was an independent fit parameter for each spectrum. The optical dispersion function of the PM6:Y6 mixture was modeled with a Kramers-Kronig constrained fixed 22 node B-Spline function.[1] For the next set of samples, the optical constant of the PM6:Y6 mixture was kept fixed. To probe the influence of aging on the optical properties of the PM6:Y6 mixture three samples identical to the above-discussed set of samples were aged for 100 h and were measured similarly.

A complete solar cell comprising of glass/ITO/ZnO/ PM6:Y6/$MoO_x$/Ag was prepared with the varying thickness of $MoO_x$ layer passivated with the Ag layer of known thickness. Once again, the MSA approach was used to determine the optical constants and thickness of the $MoO_x$ layer, while the optical constant of the Ag was used from the CompleteEASE database and the thickness of the Ag was kept fixed to 2.0 nm. The thickness of the Ag layer was determined from the quartz microbalance measurement during the deposition. Similar to the PM6:Y6 mixture, the dispersion relation of the $MoO_x$ layer was modeled with a 22 nodes B-Spline function following the Kramer-Kronig constraint. The nodes were matched to the optical constants of $MoO_3$[2] as an estimate before fitting to improve the chance of finding a correct solution.

## II. TRANSIENT ABSORPTION (TA) SPECTROSCOPY

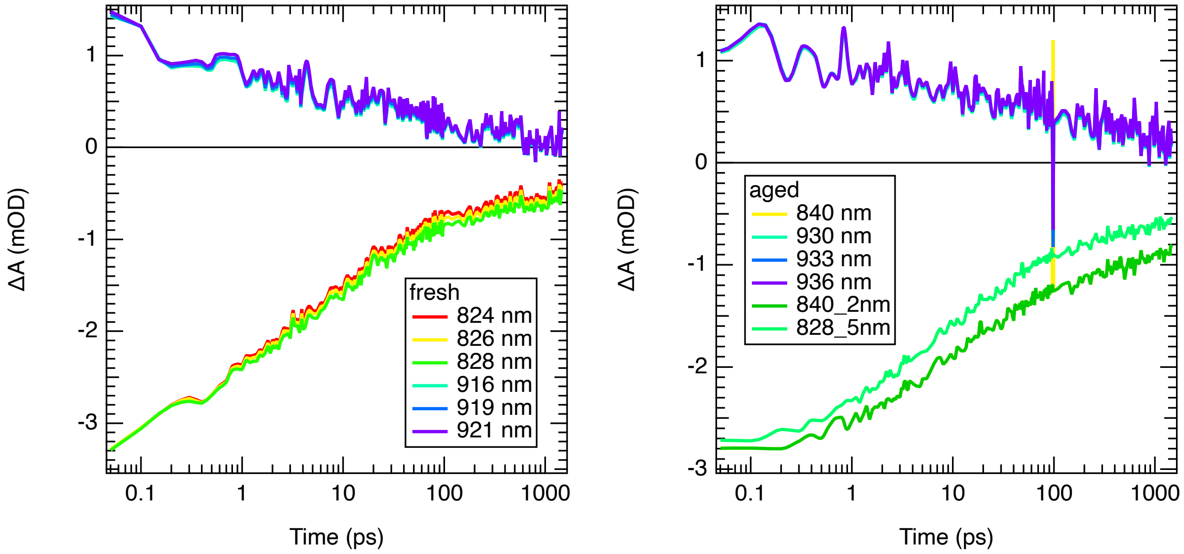


FIG. 2. Transient absorption spectroscopy of (left) fresh and (right) aged PM6:Y6 thin films.

## III. $\mathrm{EQE_{PV}}$ SUB-BANDGAP ENERGETICS

The low absorbing part of $\mathrm{EQE_{PV}}$ can be approximated by an exponential distribution of states; the slope is identified with the corresponding Urbach energy $E_\mathrm{U}$

$$\mathrm{EQE_{PV}} \propto \exp\left(\frac{E}{E_\mathrm{U}}\right) \tag{1}$$

As is shown in Fig. 3, $E_\mathrm{U}$ varies slightly between both cell thicknesses, yet remains unaffected by aging.

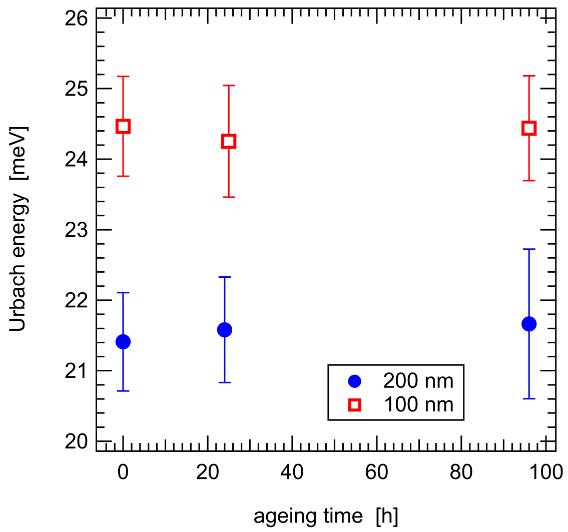


FIG. 3. Urbach energies of the sub-bandgap tail state distribution for solar cells with 100 nm and 200 nm thick active layers. Thicker cells exhibit a slightly lower Urbach energy, which in both cases remains unaffected by aging.

### A. Influence of radiative efficiency on $V_{oc}$

If the electroluminescence quantum yield $QY_{EL}$ follows a distinct temperature dependence,[3] we would expect a substantial influence on the quasi-Fermi-level splitting. From the Shockley equation with ideality factor $n \neq 1$, we find

$$QY = QY^0 J_{inj}^{n-1} \exp\left(\frac{-\Delta E}{kT}\right) \tag{2}$$

$$J_{inj} = \frac{J_0^{rad}}{QY} \exp\left(\frac{qV}{kT}\right) \tag{3}$$

$$J(V) = \left(\frac{J_0^{rad}}{QY^0}\right)^{1/n} \exp\left(\frac{\Delta E}{nkT}\right)\left(\exp\left(\frac{qV}{nkT}\right) - 1\right) - J_{sc} \tag{4}$$

Under open-circuit conditions ($J(V) = 0$), the energy barrier $\Delta E$ works as a constant difference to the radiative limit given by $J_0^{rad}$

$$qV_{oc} \approx nkT \ln(J_{sc}) - nkT \ln\left(\frac{J_0^{rad}}{QY^0}\right)^{1/n} + nkT\left(\frac{-\Delta E}{nkT}\right) \tag{5}$$

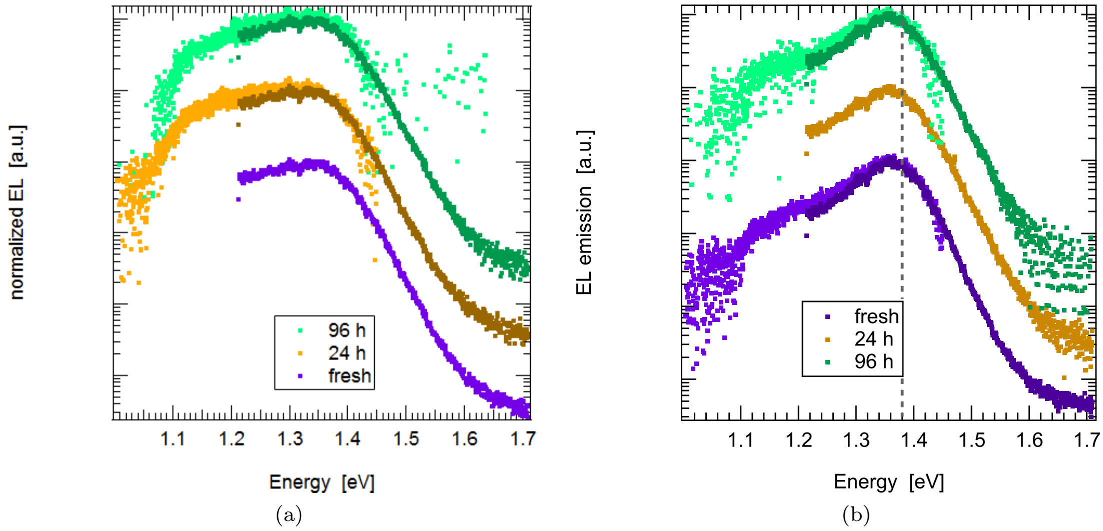


FIG. 4. Normalized electroluminescence spectra for (a) 100 nm and (b) 200 nm thick device at room temperature under constant injection current density of 96 mA cm$^{-2}$. The spectra were measured by liquid-Nitrogen cooled Indium-Gallium-Arsenide- and Silicon-cameras and were subsequently normalized to match at their maximum around 1.35 eV.

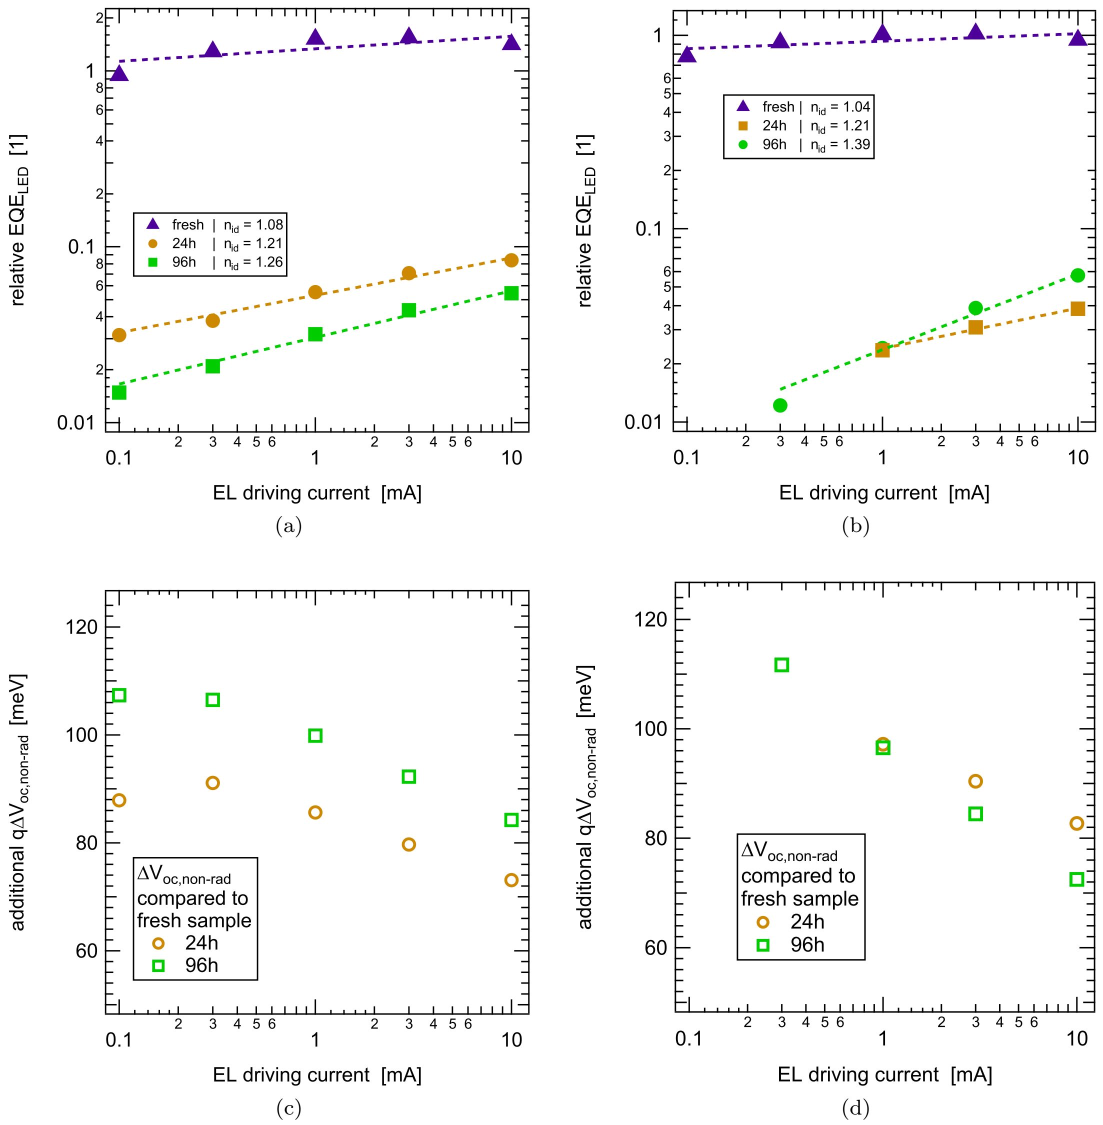


FIG. 5. Integrated electroluminescence spectra for (a) 100 nm and (b) 200 nm thick devices at room temperature and increasing injection currents. The slope of the integrated values (dashed line) corresponds to the electroluminescence ideality factor, which increases during aging. At the same time, the overall electroluminescence intensity is reduced upon aging, suggesting increased non-radiative recombination. The lower integral value corresponds to an additional non-radiative voltage loss for the (c) 100 nm and (d) 200 nm thick device. However, as the devices have to be kept under inert atmosphere for the 96 h aging procedure and are placed in a custom-build sample chamber for electroluminescence measurements, the absolute emission quantum yield could not be determined with reasonable certainty.

### B. Effective band gap

Recently, it was found from electroluminescence measurements that while overall recombination in PM6:Y6 occurs non-radiatively from CT states, the radiative recombination is dominated by $S_1$ states in Y6, which are repopulated via an energy barrier of $\Delta E_{\mathrm{S_1\text{-}CS}} \approx 117$ meV.[3] As a result, the EL quantum yield is temperature dependent with an exponential dependency on $\Delta E_{\mathrm{S_1\text{-}CS}}$ and $kT$.

The repopulation of $S_1$ states causes a reduced quasi-Fermi-level splitting of the charge-separated states at high temperatures. According to Eqn. (**??**), this energy loss can be attributed to the energy barrier $\Delta E_{\mathrm{S_1\text{-}CS}}$ and affects the measured $V_{\mathrm{oc}}$ of the device:

$$\mathrm{QY_{EL}} = \mathrm{QY_{EL}^0} \exp\left(-\frac{\Delta E_{\mathrm{S_1\text{-}CS}}}{kT}\right) \tag{6}$$

$$eV_{\mathrm{oc}} \approx n_{\mathrm{id}} kT \ln\left(J_{\mathrm{sc}}\right) - kT \ln\left(\frac{J_0^{\mathrm{rad}}}{\mathrm{QY_{EL}^0}}\right) - \Delta E_{\mathrm{S_1\text{-}CS}} \tag{7}$$

The extrapolated limit of $V_{\mathrm{oc}}$ to 0 K, $E_{\mathrm{g,eff}}$, is therefore always lower than the (ideal) radiative quasi-Fermi-level splitting (QFLS) suggests, and $\Delta E_{\mathrm{S_1\text{-}CS}}$ can be expressed as a temperature-independent part of the non-radiative $V_{\mathrm{oc}}$ losses ($kT \ln\left(\mathrm{QY_{EL}}\right)$). While the QFLS limit was found at 1.1 eV, the corrected effective bandgap (defined by the limit of the radiative recombination current $J_0^{\mathrm{rad}}$ and $QY_{\mathrm{EL}}^0$) is located at $E_{\mathrm{g,eff}} + \Delta E_{\mathrm{S_1\text{-}CS}} \approx 1.22$ eV according to Eqn. (6). However, the origin of the remaining difference of 160 meV between the effective band gap and the optical band gap still remains unclear.

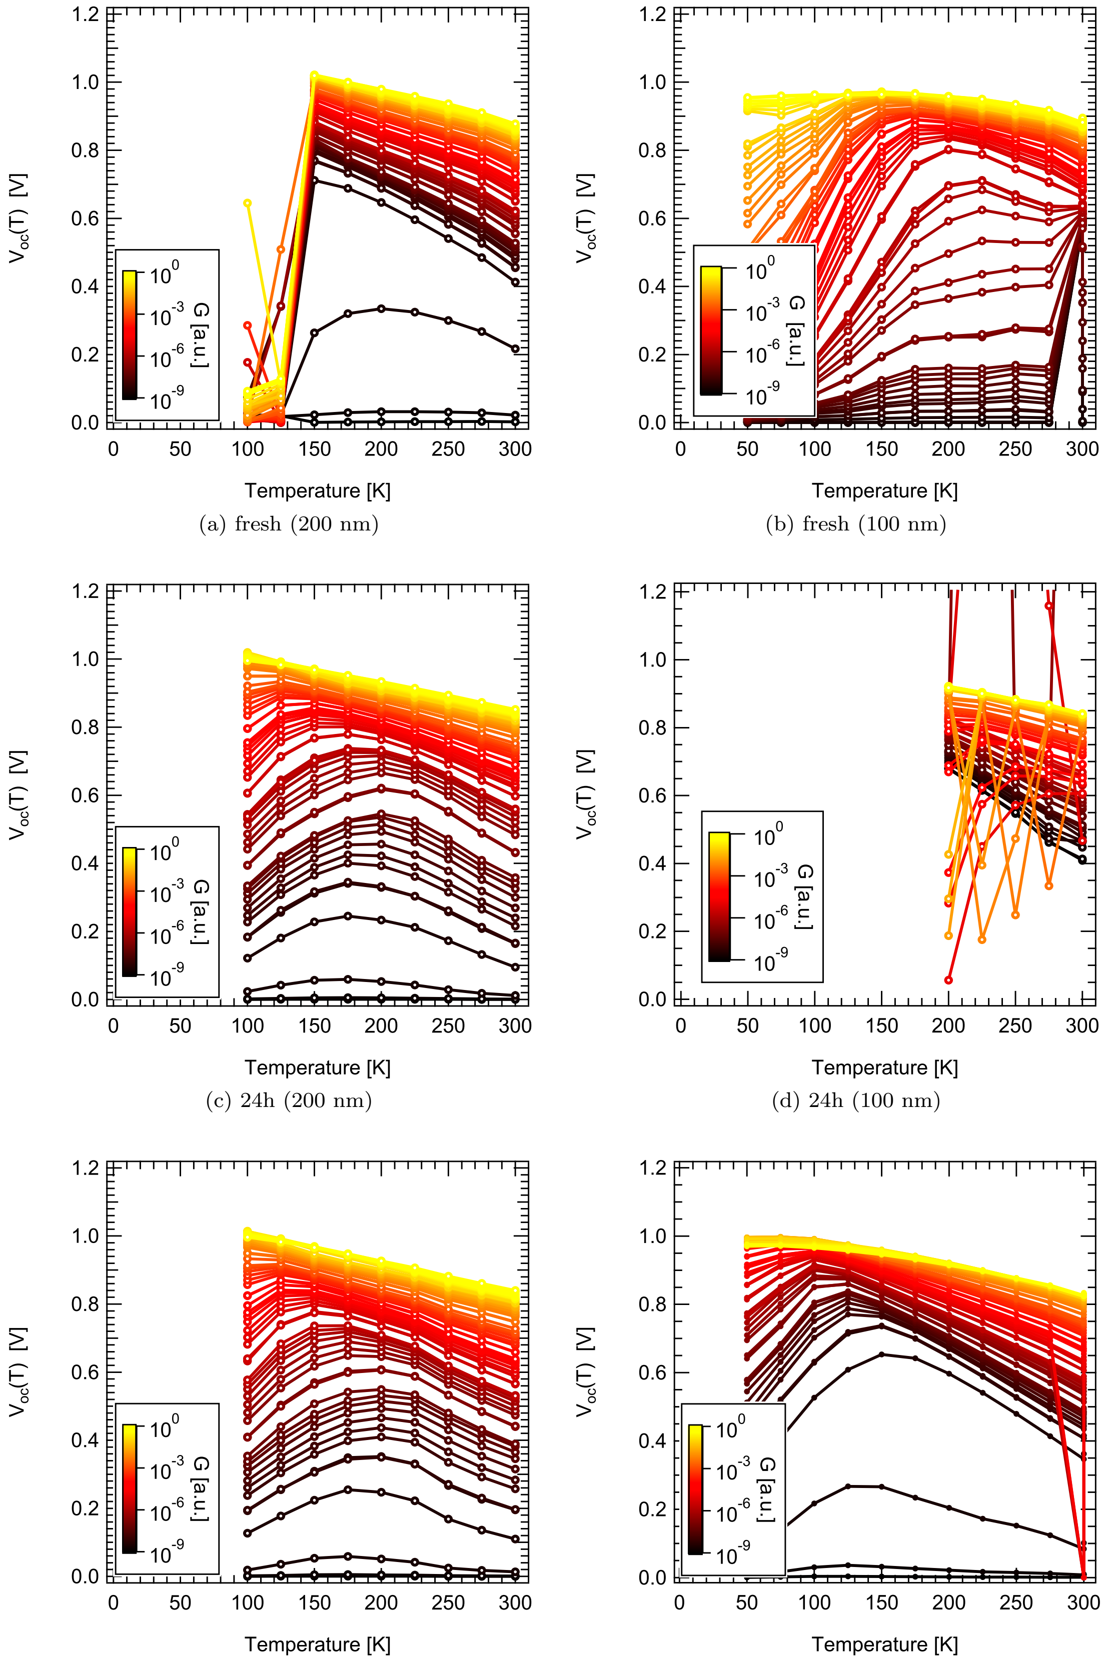


(a) fresh (200 nm)

(b) fresh (100 nm)

(c) 24h (200 nm)

(d) 24h (100 nm)

(e) 96h (200 nm)

(f) 96h (100 nm)

FIG. 6. Open circuit voltages $V_{\rm oc}$ for temperature $T$ and for 9 orders of magnitude of generation rate $G$ of thick and thin devices at various aging steps. The measured values are shunt-limited at very low generation rates, and contact issues occur in the custom-built cryostat at low temperatures.

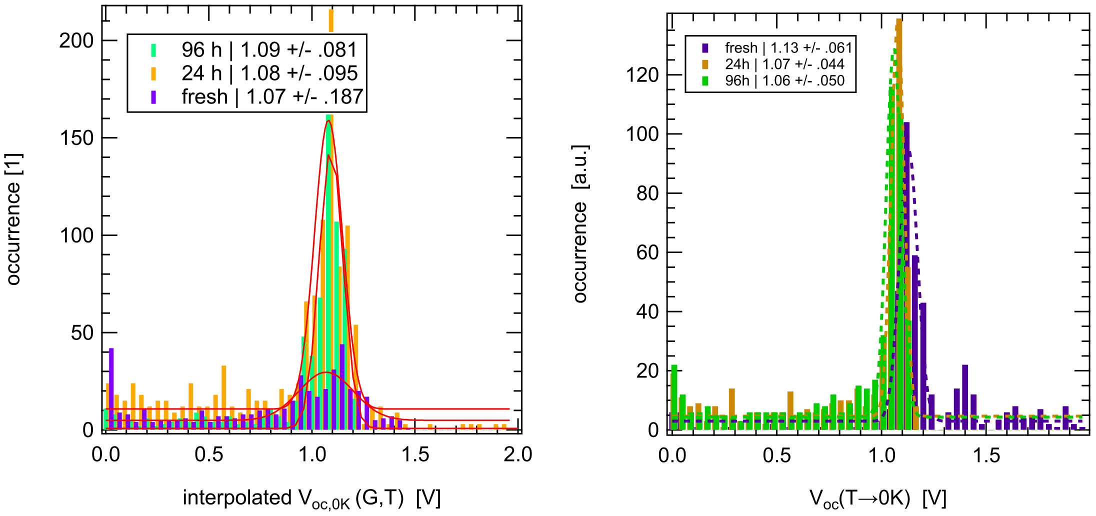


(a) (b)

FIG. 7. Histograms of open-circuit voltages (Fig. 6), locally linear extrapolated to $T = 0$ K, of (a) 100 nm and (b) 200 nm thick devices at different aging steps. The histograms were fitted with a normal distribution to determine the low temperature limit of the open-circuit voltage. Values for the limit and uncertainties from the distribution width are given in the annotations; no significant change is caused by the aging process.

## IV. CONDUCTIVITY

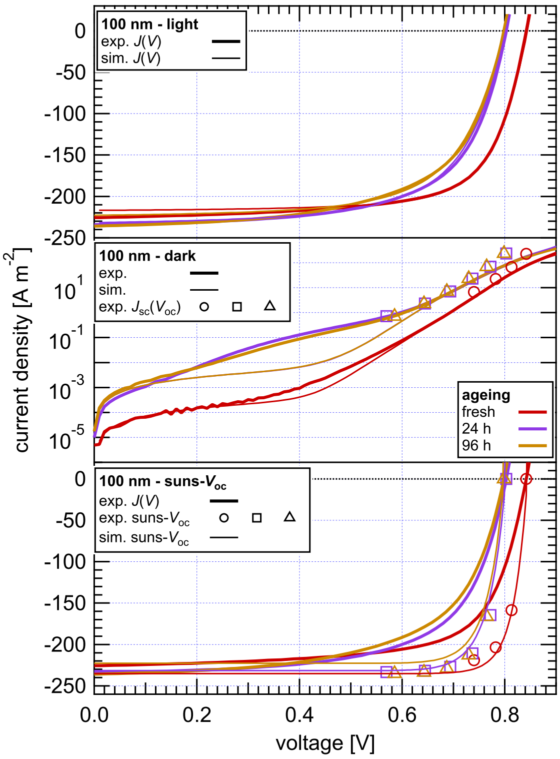


FIG. 8. Current–voltage characteristics of fresh and aged solar cells with an active-layer thickness of 100 nm. (Top) Experimental and simulated $JV$ curves under 1-sun equivalent illumination. (Center) Experimental $JV$ curves in the dark and $J_{\rm sc}(V_{\rm oc})$ data as well as simulated $JV$ curves in the dark. The experimental data show a parasitic feature at the transition from the shunt resistance-dominated part to the exponential part ranging from 0.1 to 0.6 V. Although its origin is unknown, we assign it to sample-to-sample variation, as other pixels on the same substrate did not show such behavior. Therefore, data in the voltage region mentioned above were excluded from the simulation. (Bottom) The same experimental $JV$ curves as in the top graph together with experimental and simulated suns-$V_{\rm oc}$ data, showing a significant voltage difference $\Delta V$ between $JV$ and suns-$V_{\rm oc}$ data at a given current density. The conductivity $\sigma$ extracted from $\Delta V$ is 9.4, 8.1 and $6.5 \cdot 10^{-5}$ S m$^{-1}$ for aging durations of 0, 24, and 96 h, respectively.

## V. CAPACITANCE–VOLTAGE MEASUREMENTS

We evaluated experimental $CV$ curves to achieve the effective charge carrier density $n$ as well as an estimate for the intrinsic charge carrier density $n_\mathrm{i}$ under open-circuit conditions.

Recently, several commonly used approaches for estimating $n\left(V_\mathrm{sat}\right)$ and $C_\mu$ were compared.[4] We chose to determine $n\left(V_\mathrm{sat}\right)$ and $C_\mu$ by

$$C_\mu\left(V\right) = C\left(V\right) - C_\mathrm{geo} \tag{8}$$

$$n\left(V_\mathrm{sat}\right) = \frac{1}{eL}\left(V_\mathrm{oc} - V_\mathrm{sat}\right) \tag{9}$$

with $C_\mathrm{geo}$ being the geometrical capacitance. $V_\mathrm{sat}$ is a voltage in the reverse-bias regime, where non-geminate recombination is heavily suppressed. $n$ is obtained from the chemical capacitance $C_\mu\left(V\right)$ using the equation

$$n\left(V_\mathrm{oc}\right) = n\left(V_\mathrm{sat}\right) + \frac{1}{eL}\int_{V_\mathrm{sat}}^{V_\mathrm{oc}} C_\mu\left(V\right)\mathrm{d}V \quad . \tag{10}$$

With $n$ being known as a function of $V_\mathrm{oc}$, the ideality factor $n_n$ of charge carrier density is calculated. Since $n\left(V_\mathrm{oc}\right)$ follows[5]

$$n = n_0 \exp\left(\frac{eV_\mathrm{oc}}{n_n kT}\right) \quad , \tag{11}$$

we can determine $n_n$ by locally deriving the natural logarithm of $n$.

With $n\left(V_\mathrm{oc}\right)$ being known we achieve an estimate for $n_\mathrm{i}$ of the active layer blend[6]

$$n_\mathrm{i} = n\left(V_\mathrm{oc}\right)\exp\left(-\frac{eV_\mathrm{oc}}{2kT}\right) \quad . \tag{12}$$

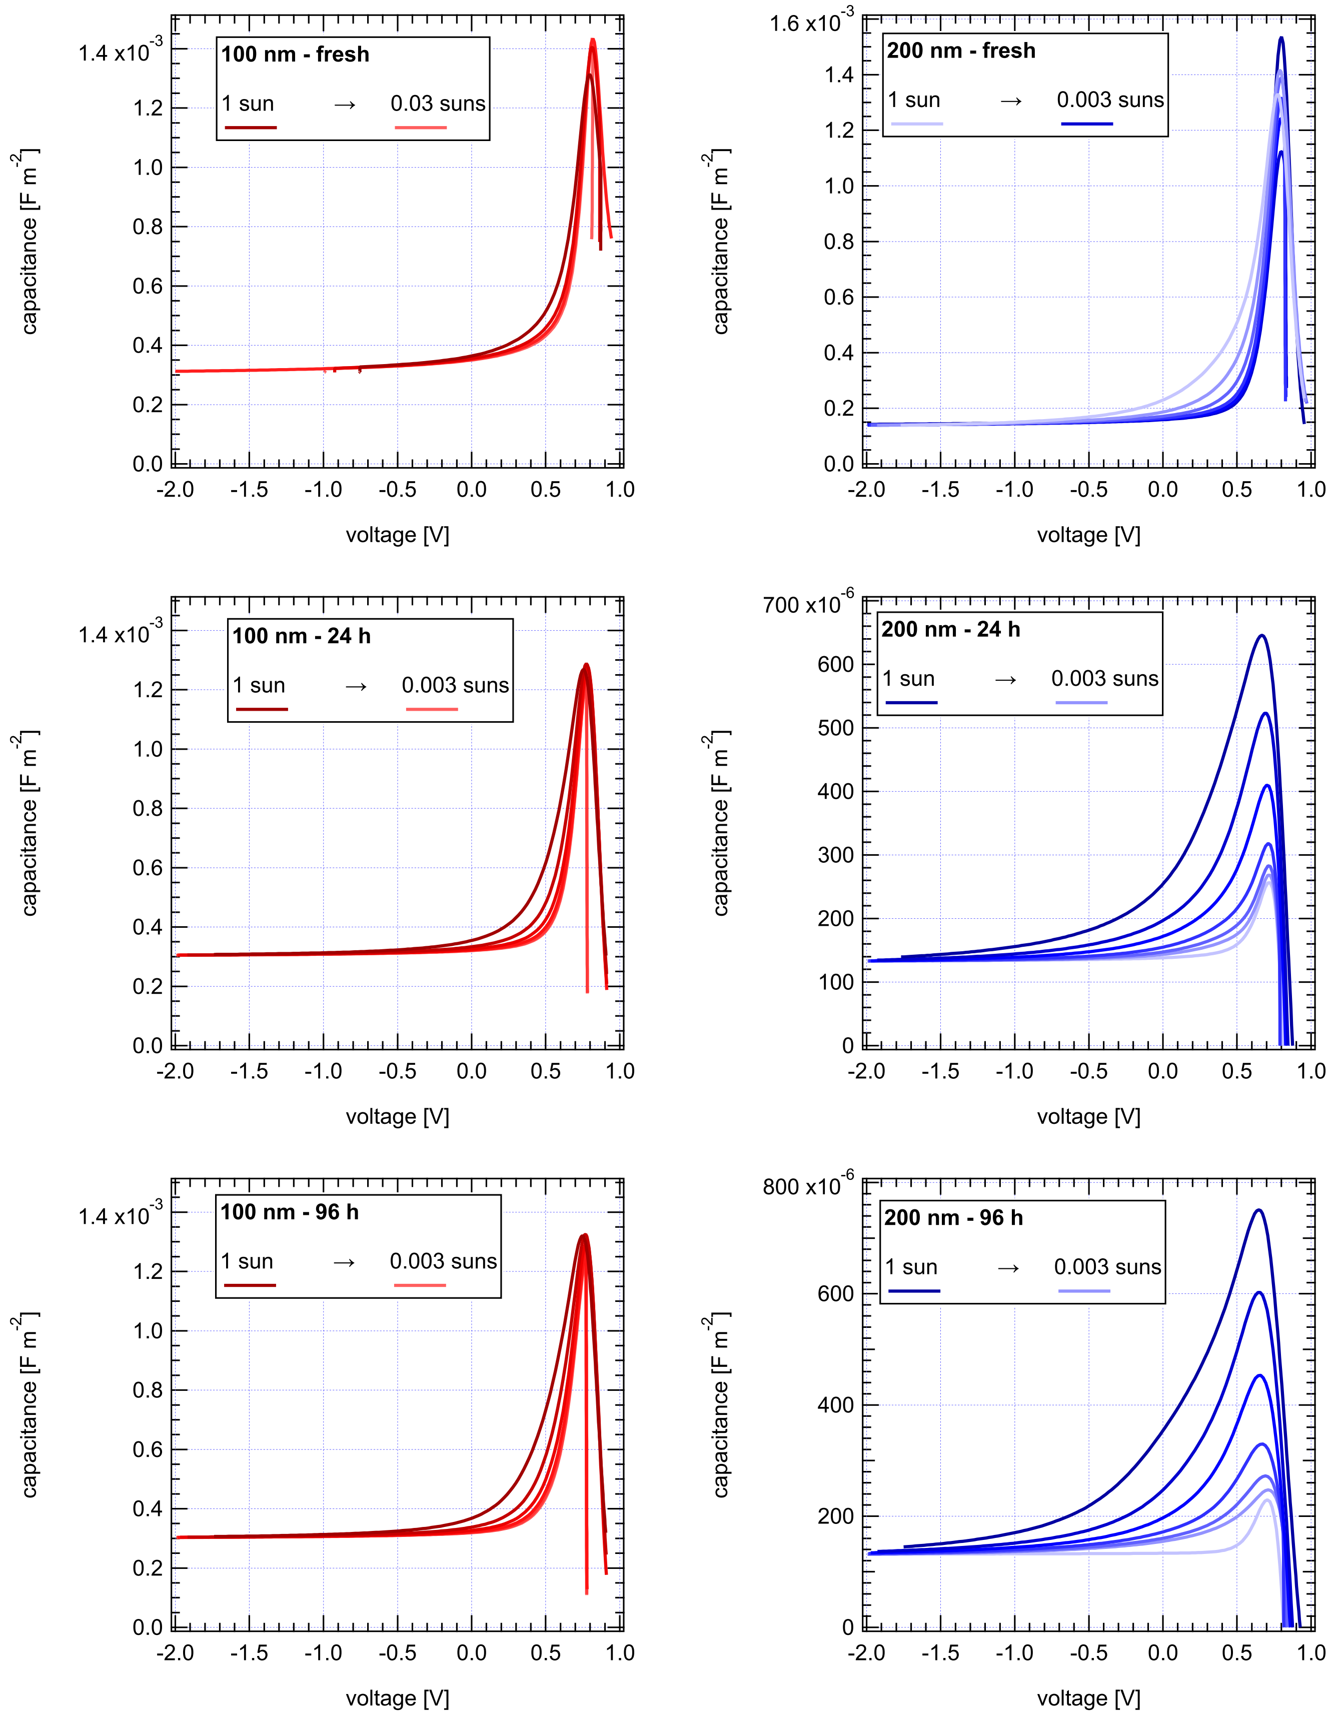


FIG. 9. Capacitance–Voltage ($CV$) measurements at subsequent aging steps on samples with different active-layer thicknesses.

## VI. INTENSITY-MODULATED SPECTROSCOPY

The Nyquist representations of IMVS data (Fig. 10) generally show one complete semicircle in the second quadrant and one incomplete semicircle in the third quadrant, both exhibiting decreasing radii with decreasing illumination intensity. The incomplete semicircles, occurring at small frequencies of 1 to 10 Hz, are attributed to parasitic effects, most probably originating from the setup and therefore ignored in the evaluation.

In the Bode representation (Fig. 10) of the IMVS real part, a plateau occurs at intermediate angular frequencies between 100 and 1000 Hz. Because the imaginary part at such small frequencies is almost zero, the real part can be used as an approximation for the voltage response $V_{\mathrm{AC}}$ to the modulated intensity amplitude $G_{\mathrm{AC}}$, which we chose to be 10 % of the bias illumination amplitude $G$. The diode ideality factor $n_{\mathrm{id}}$ can be calculated from the IMVS real part according to Eqn. (1) in the main text.

The effective small-perturbation charge-carrier lifetime $\tau_{\Delta n}$ is extracted from the angular frequency, at which the imaginary part of the IMVS occurs. With the recombination order $\lambda$ (see below) this can be transformed into the effective charge-carrier lifetime $\tau_n = (\lambda + 1)\,\tau_{\Delta n}$ shown in Fig. 11. Both $\tau_{\Delta n}$ and $\tau_n$ follow[5]

$$\tau_n = \tau_{n,0} \exp\left(-\frac{eV_{\mathrm{oc}}}{n_\tau kT}\right) \quad . \tag{13}$$

From here, the lifetime ideality factor $n_\tau$ is calculated by locally deriving the natural logarithm of the above equation. The results are shown in Fig. 11. For moderate and small illumination intensities below 0.1 suns, $n_\tau$ is generally dropping with aging, ranging from 2.3 for the fresh device to 1.8 for the 96 h aged one. At higher illumination intensities approaching 1 sun, $n_\tau$ drops below 1.5 for all aging steps studied here, which we again attribute to surface recombination. At 0.1 suns and below $n_\tau$ approaches and saturates around a value of 2.

### A. The recombination ideality factor

The recombination ideality factor $n_{\mathrm{R}}$, which was shown to be equal to $n_{\mathrm{id}}$,[5] is calculated as the harmonic mean of $n_n$ and $n_\tau$. Then, $n_{\mathrm{R}}$ is compared to $n_{\mathrm{id}}$ calculated from IMVS (Fig. 11). Although both ideality factors are not exactly equal, they display a comparable trend: $n_{\mathrm{R}}$ decreases with increasing illumination intensity, starting at approximately 1.4 for 0.003 suns and approaching unity at 0.1 suns for all aging steps. At illumination intensities above 0.3 suns, it drops below 1, which is again assigned to surface recombination becoming dominant.

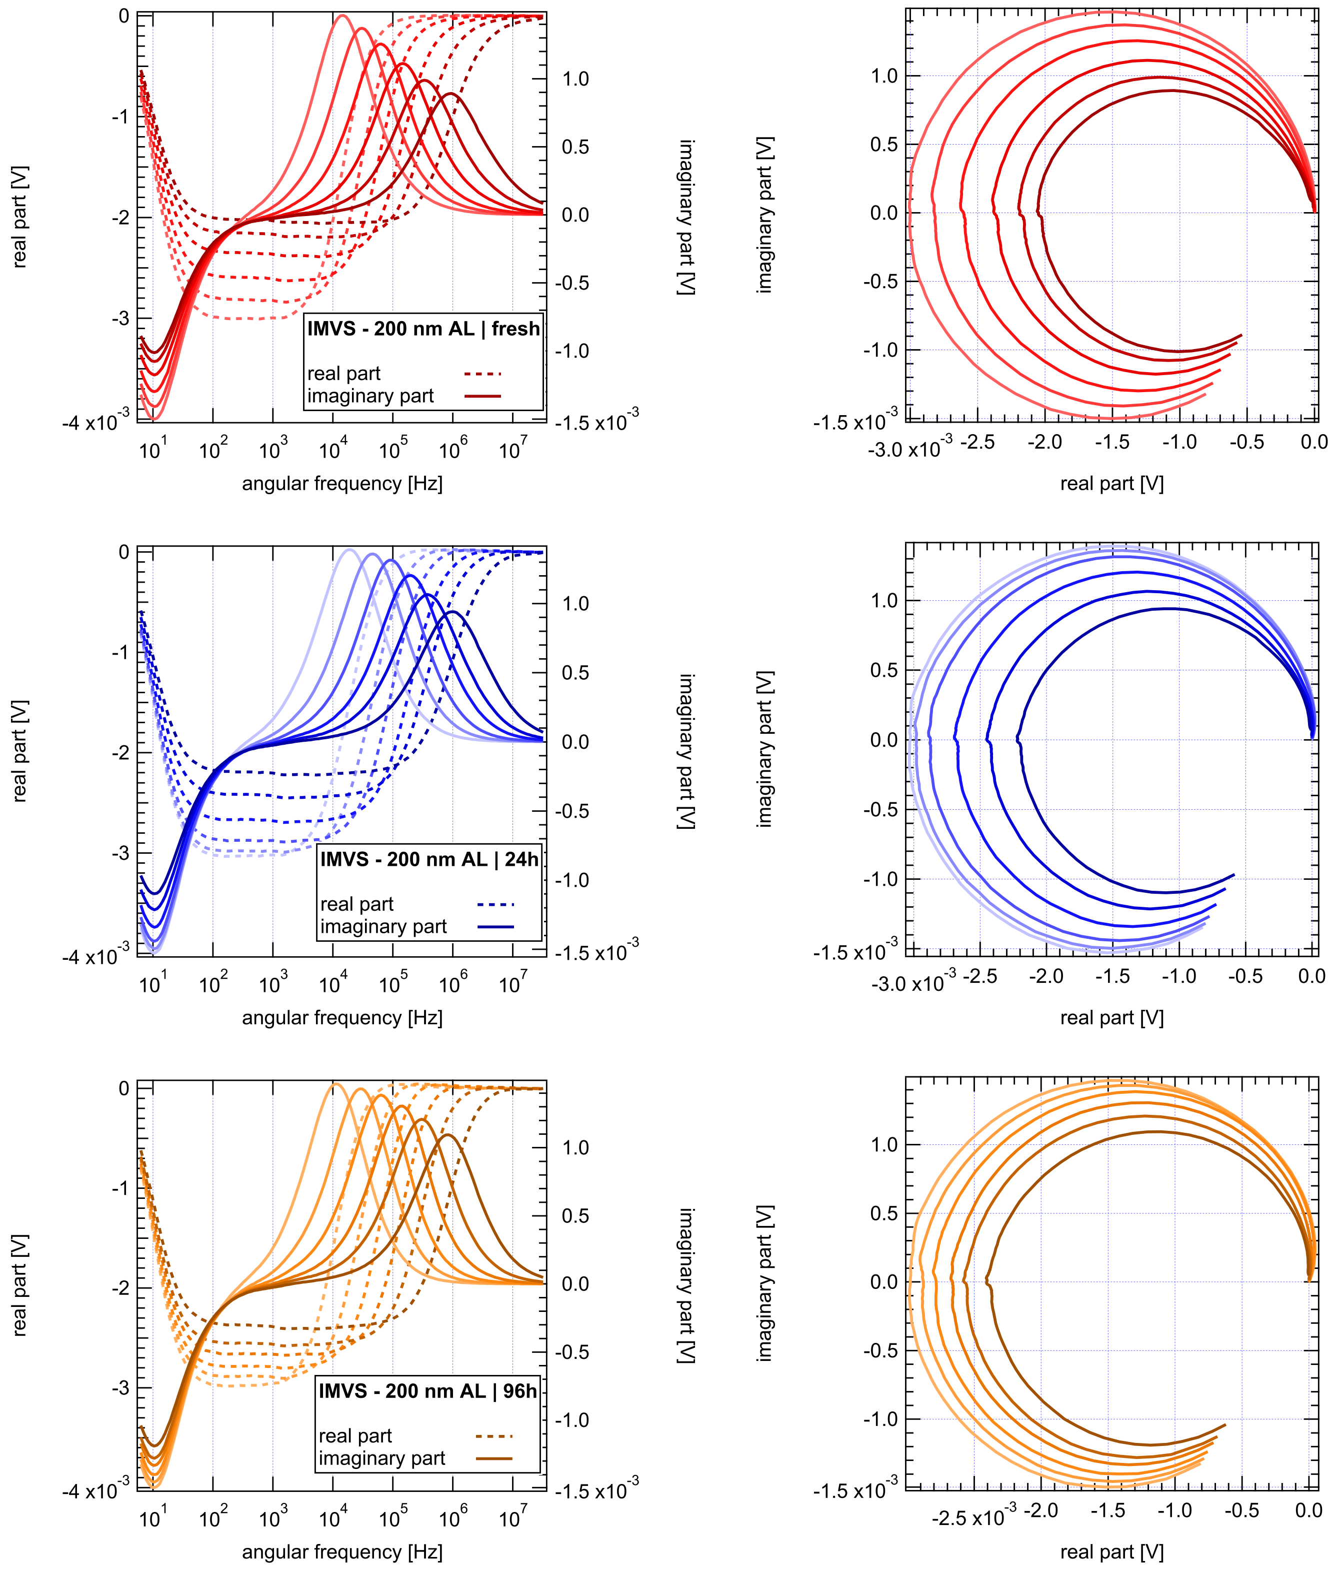


FIG. 10. IMVS raw data in (left) Bode and (right) Nyquist representation.

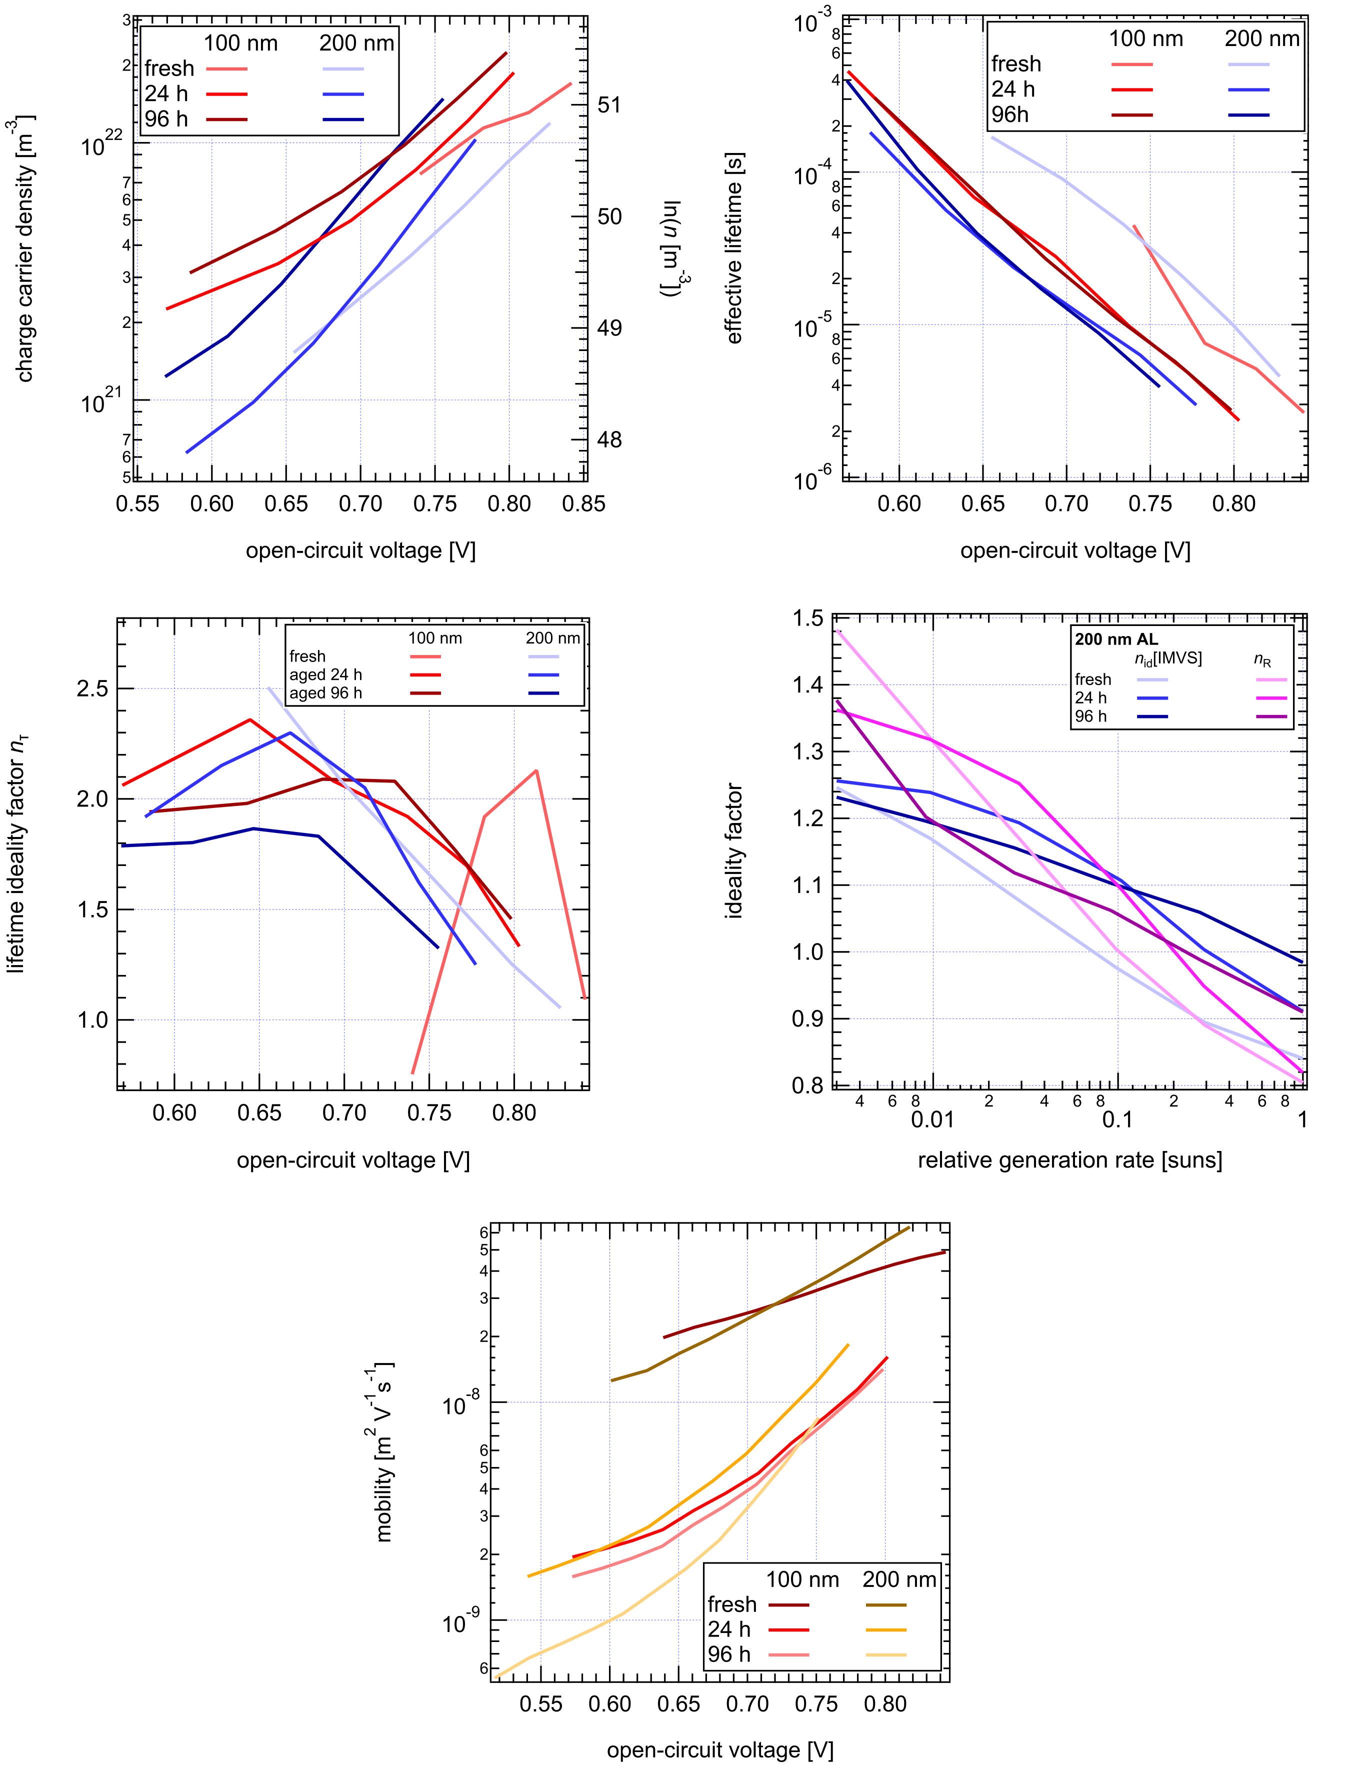


FIG. 11. (Top left) Effective charge-carrier density $n$. (Top right) effective charge carrier lifetime $\tau_n$ for subsequent aging steps. (Center left) $n_\tau$ extracted from the measurements of $\tau_n$. (Center right) device ideality factor $n_{\rm id}$ and recombination ideality factor $n_{\rm R}$ for the thick device. (Bottom left) Simulated charge carrier mobility.

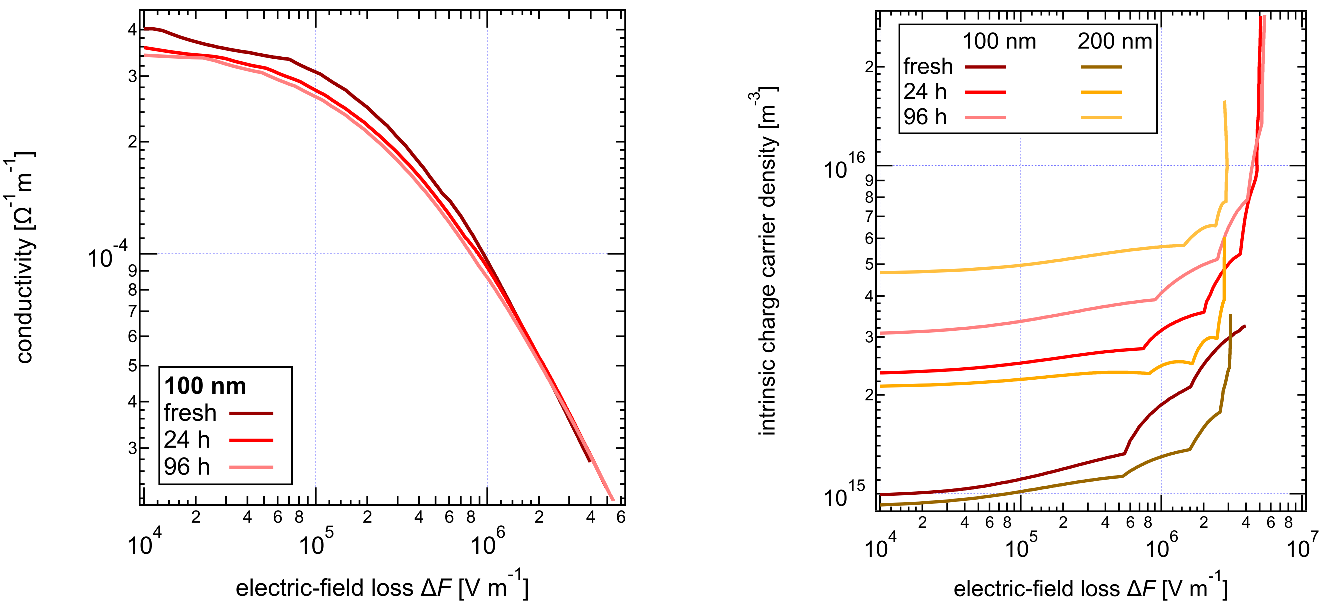


FIG. 12. (Left) Effective conductivity $\sigma$ of the device with 100 nm thick active layer, (right) intrinsic charge carrier density $n_\mathrm{i}$. The electric-field screening $\Delta F$ is determined from $JV$ measurements under 1 sun-equivalent monochromatic illumination and suns–$V_\mathrm{oc}$ measurements for each current density.

## VII. GRAZING INCIDENCE WIDE ANGLE X-RAY SCATTERING (GIWAXS)

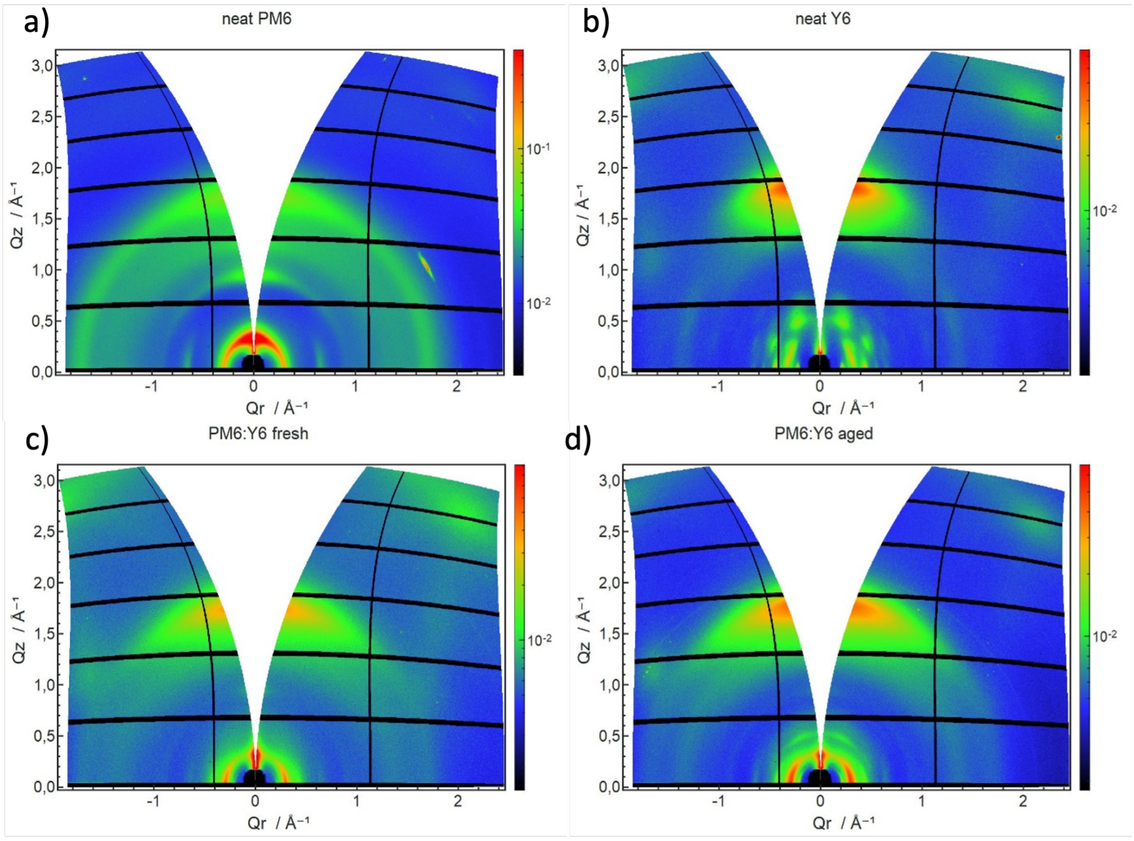


FIG. 13. q-converted 2D GIWAXS data for a) PM6, b) Y6, c) PM6:Y6 fresh and d) PM6:Y6 aged for 96 h spincoated on silicon substrates. Vertical information along $q_z$ (region around the vertical gap) includes information about orientation perpendicular to substrate, whereas horizontal information along $q_r$ holds information on orientation parallel to the substrate.

The samples of neat PM6 and neat Y6 thin films spincoated on silicon substrates show each high ordering in the 2D GIWAXS data (Fig. 13a and b). Upon blending both materials, the GIWAXS data shows a reduction in the long range ordering for both materials (Fig. 13c). However, during the implemented ageing process both material components recover some of their neat material order signatures (Fig. 13d). Particularly for the Y6 the peaks observed in the lower q-range indicate that several molecules must arrange in lateral and vertical direction.

The $q$-converted 2D GIWAXS data for a) PM6, b) Y6, c) PM6:Y6 fresh and d) PM6:Y6 aged for 96 h on ITO/ZnO are shown in Fig. 14. In contrast to the PM6:Y6 blends prepared on silicon substrates the ones prepared on ITO coated with ZnO show already weaker ordering for the neat materials (Fig. 14a and b) and a much weaker dependence on aging (Fig. 14c to d). The $\pi$–$\pi$-peak of the neat PM6 is a Lorentzian with $q_{z,f}$ = (16.70 ± 0.02) nm$^{-1}$ with a real space distance of $d_{v,f}$ = (3.762 ± 0.006) Åand the $\pi$–$\pi$-peak of the neat Y6 is a Lorentzian with $q_{z,f}$ = (17.36 ± 0.04) nm$^{-1}$ with a real space distance of $d_{v,f}$ = (3.619 ± 0.009) Å. The $\pi$–$\pi$-peak of the blend can be fit with a variety of combinations of these two peak contributions depending of the allowed degrees of freedom (peak height, peak width, peak position). In all cases the PM6 contribution dominates strongly and shows a clear change from a more well defined Lorentz to a broader peak after 96 h of artificial aging.

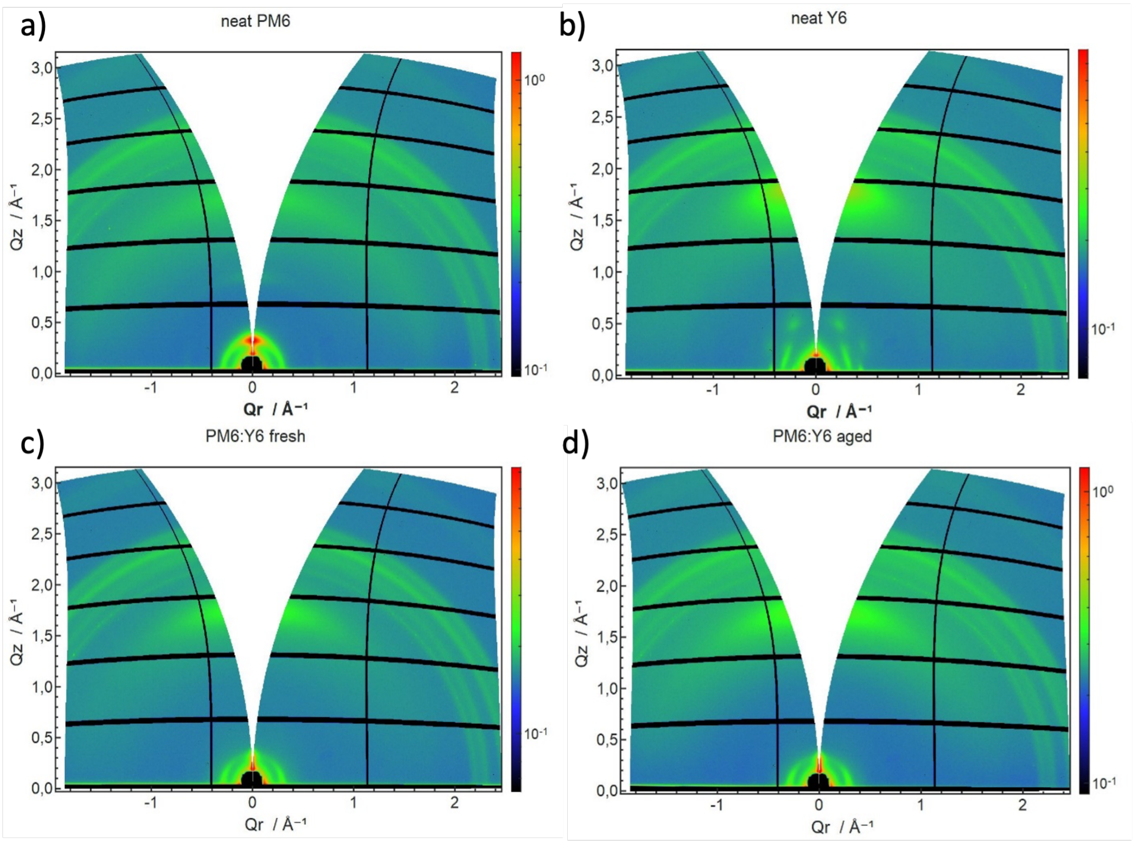


FIG. 14. $q$-converted 2D GIWAXS data for a) PM6, b) Y6, c) PM6:Y6 fresh and d) PM6:Y6 aged for 96 h spincoated on ITO/ZnO coated glass substrates. 1D intensity data (Fig. 1c) was extracted with two cuts, containing horizontal and vertical information. Vertical information (15°azimuthal integration around the vertical gap) includes information about orientation perpendicular to substrate, whereas horizontal information (15°azimuthal integration parallel to $x$-axis) holds information on orientation parallel to the substrate.

## VIII. ULTRAVIOLET PHOTOEMISSION SPECTROSCOPY (UPS)

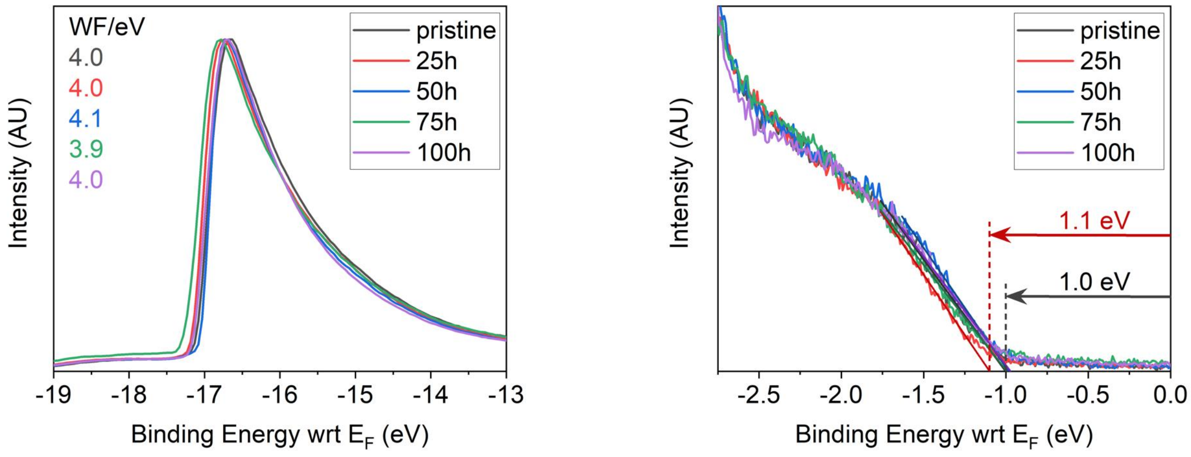


FIG. 15. UPS traces on surfaces of fresh (pristine) and aged samples.

# IX. DETAILS OF THE DEVICE SIMULATION

## A. The model

The details of the device model were described elsewhere, in short the model solves the drift–diffusion equations, Poisson's equation, and the Shockley-Read-Hall (SRH) trapping and escape equations. It is important to note that the SRH capture escape equations are solved explicitly. This means that the device is discretized in position space using a finite difference mesh, the transport and drift diffusion equations are solved on this mesh between the contacts. Under each mesh point in position space, energy space is also discretized, meaning the LUMO and HOMO are split up into 5-10 distinct energy levels. For each of these energy ranges a SRH capture escape equation is solved. The capture escape rates are calculated before the simulation begins by integrating the SRH functions over the exponential distribution of trap states for each energy range, then tabulating them as a function of trap Fermi level and free carrier Fermi level. This approach allows dynamic carrier events to be simulated, which is distinctly different to simply solving the analytical SRH equation already integrated over energy space at each mesh point.

## B. Extension of the model to frequency domain

Previously the general approach to solving frequency domain problems was to solve the DC problem then cast the same set of equations into a small signal form,[7] solve these and add the two results. This approach although efficient has two drawbacks. The first is casting the Jacobian into a small signal form is often nontrivial to do, and one effectively ends up maintaining two Jacobians, one DC/time domain form and one small signal one. The second issue with this approach is that it is not clear when/where the linear approximation is valid, this is an especially relevant concern when one is dealing with a non-linear set of traps. Considering the progress in multi-core computers since the work by Laux,[7] we decided for this work to model the frequency domain by solving the set of equations in the time domain for each frequency of interest. Therefore to simulate impedance spectroscopy voltage perturbations were applied to the time domain model and the resulting current examined. Each simulation is run on its own thread in parallel.

## C. Extracting phase information from AC signals

Extracting real and imaginary phase information from simulated AC signals is not straightforward, because the signal is comprised of a finite number of points. To extract the phase information exactly, one would need a very fine time step, which would be costly to simulate. Instead in this work, we used as few time domain points as necessary to simulate the signal accurately, then extract the real and imaginary parts by fitting a perfect sine wave to the simulated AC output/input signals.

The fit is performed by first taking the discrete Fourier transform of the signals to get an estimate of the phase and magnitude, the result is not accurate due to the non-infinite nature of the signal. We then use the phase information to guess where to place the sine functions on top of the simulated data to get a good fit. Newton's method is then used to optimize the magnitude, phase, and DC offset in turn.

## D. Fitting to experimental data

Tables I and II show the simulation parameters for the 100 nm and 200 nm thick devices. Values below the horizontal line were constants, those above the line were allowed to vary. The results of the fits can be seen in Figs. 16–18 for the 100 nm device and in Figs. 19–21 for the 200 nm device. The quality of the fit was prioritized in the following order: dark $JV$ curve, light $JV$ curve, $CV$, Suns-$V_{\mathrm{oc}}$, impedance spectroscopy data. The downhill simplex algorithm was used for the fitting, each simulation (including each frequency domain point) was run of an individual thread.

TABLE I. Simulation parameters for an active-layer thickness of 200 nm.

| Parameter | 0 h | 24 h | 96 h | Units |
|---|---|---|---|---|
| Electron trap density | $1.1 \times 10^{25}$ | $2.6 \times 10^{25}$ | $3.3 \times 10^{25}$ | $m^{-3}$ $eV^{-1}$ |
| Hole trap density | $6.7 \times 10^{23}$ | $1.3 \times 10^{25}$ | $1.6 \times 10^{25}$ | $m^{-3}$ $eV^{-1}$ |
| Free hole to Trapped electron | $9.6 \times 10^{-23}$ | $3.9 \times 10^{-23}$ | $2.6 \times 10^{-23}$ | $m^{-2}$ |
| Free electron to Trapped hole | $1.3 \times 10^{-23}$ | $3.9 \times 10^{-23}$ | $2.6 \times 10^{-23}$ | $m^{-2}$ |
| Free hole to Trapped hole | $2.8 \times 10^{-21}$ | $1.6 \times 10^{-21}$ | $1.9 \times 10^{-21}$ | $m^{-2}$ |
| Free electron to Trapped electron | $1.3 \times 10^{-23}$ | $1.6 \times 10^{-21}$ | $1.9 \times 10^{-21}$ | $m^{-2}$ |
| Series resistance | 0.270 | 0.161 | 5.956 | *Ohms* |
| Contact charge density | $2.4 \times 10^{23}$ | $1.2 \times 10^{23}$ | $1.2 \times 10^{23}$ | $m^{-3}$ |
| Charge carrier mobility | $6.8 \times 10^{-08}$ | $1.3 \times 10^{-07}$ | $1.5 \times 10^{-07}$ | $m^2V^{-1}s^{-1}$ |
| Electron tail slope | 0.065 | 0.065 | 0.065 | $eV$ |
| Hole tail slope | 0.075 | 0.075 | 0.075 | $eV$ |
| Photon efficiency | 0.677 | 0.704 | 0.674 | $0 - 1$ |
| Shunt resistance | $1.4 \times 10^{03}$ | 80.000 | 80.000 | $Ohmsm^2$ |
| $E_g$ | 1.250 | 1.250 | 1.250 | $eV$ |

TABLE II. Simulation parameters for an active-layer thickness of 100 nm.

| | | | | |
|---|---|---|---|---|
| Electron trap density | $1.9 \times 10^{24}$ | $2.3 \times 10^{25}$ | $6.8 \times 10^{25}$ | $m^{-3}$ $eV^{-1}$ |
| Hole trap density | $2.5 \times 10^{24}$ | $1.2 \times 10^{25}$ | $2.7 \times 10^{25}$ | $m^{-3}$ $eV^{-1}$ |
| Free hole to Trapped electron | $3.0 \times 10^{-25}$ | $6.0 \times 10^{-23}$ | $4.1 \times 10^{-23}$ | $m^{-2}$ |
| Free electron to Trapped hole | $3.2 \times 10^{-23}$ | $6.0 \times 10^{-23}$ | $4.1 \times 10^{-23}$ | $m^{-2}$ |
| Free hole to Trapped hole | $3.8 \times 10^{-18}$ | $1.3 \times 10^{-21}$ | $9.4 \times 10^{-21}$ | $m^{-2}$ |
| Free electron to Trapped electron | $1.2 \times 10^{-22}$ | $1.3 \times 10^{-21}$ | $9.4 \times 10^{-21}$ | $m^{-2}$ |
| Series resistance | 0.015 | 0.357 | 4.276 | *Ohms* |
| Contact charge density | $8.1 \times 10^{22}$ | $8.1 \times 10^{22}$ | $8.1 \times 10^{22}$ | $m^{-3}$ |
| Charge carrier mobility | $1.1 \times 10^{-07}$ | $2.1 \times 10^{-07}$ | $2.8 \times 10^{-07}$ | $m^2V^{-1}s^{-1}$ |
| Electron tail slope | 0.065 | 0.065 | 0.065 | $eV$ |
| Hole tail slope | 0.075 | 0.075 | 0.075 | $eV$ |
| Photon efficiency | 0.645 | 0.648 | 0.692 | $0 - 1$ |
| Shunt resistance | 500.000 | 130.000 | 300.000 | $Ohmsm^2$ |
| $E_g$ | 1.250 | 1.250 | 1.250 | $eV$ |

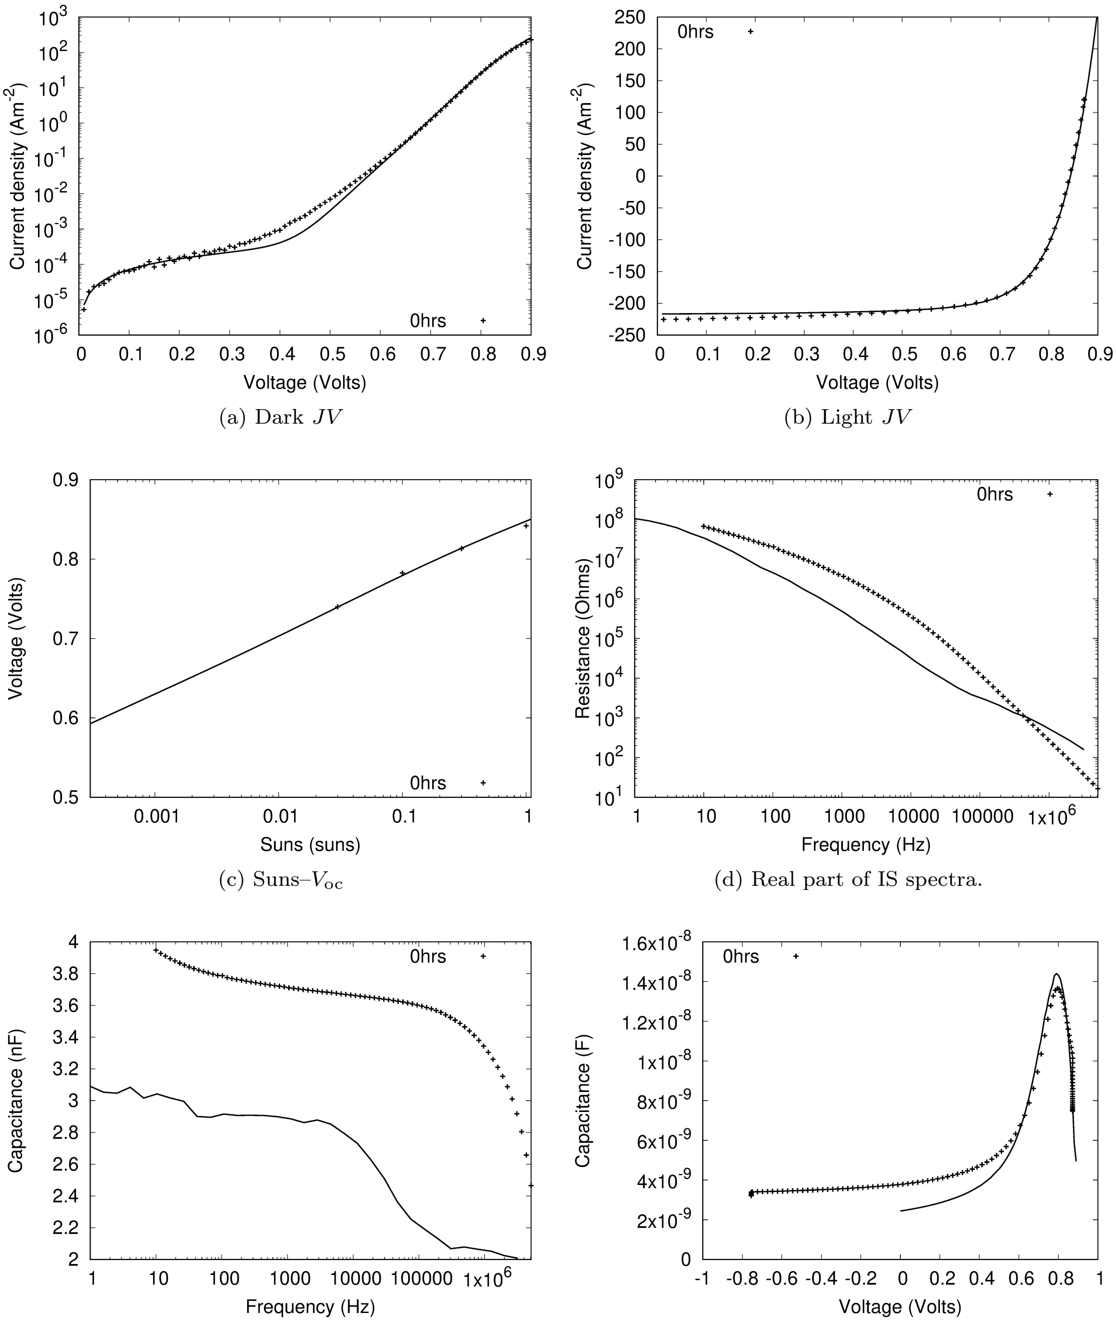


(a) Dark $JV$

(b) Light $JV$

(c) Suns–$V_{oc}$

(d) Real part of IS spectra.

(e) Imaginary part of IS spectra.

(f) Capacitance–Voltage

FIG. 16. Fits of the model to the 100 nm device at 0 h

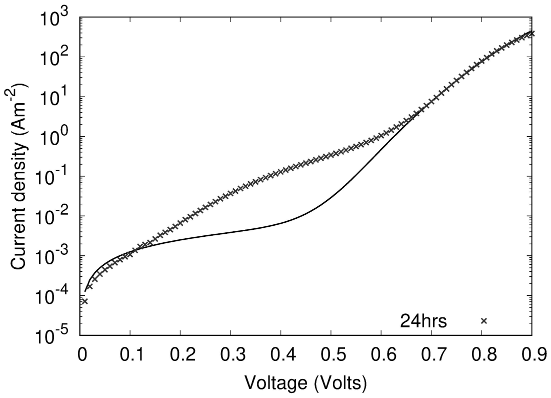


(a) Dark $JV$

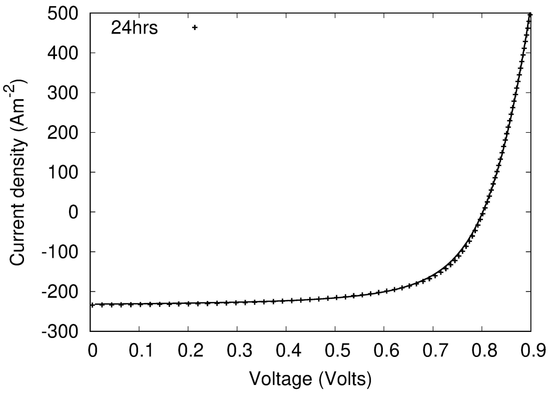


(b) Light $JV$

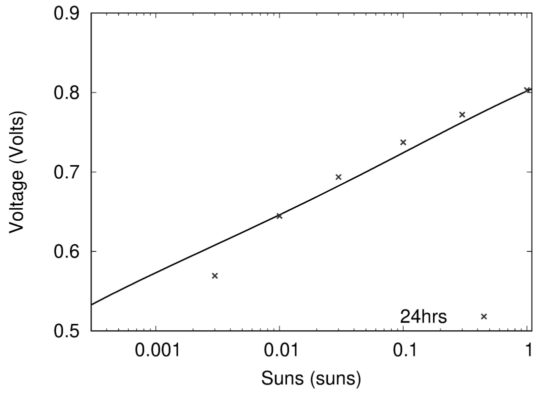


(c) Suns–$V_{oc}$

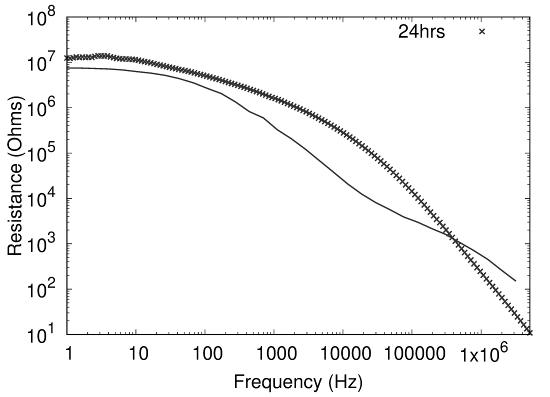


(d) Real part of IS

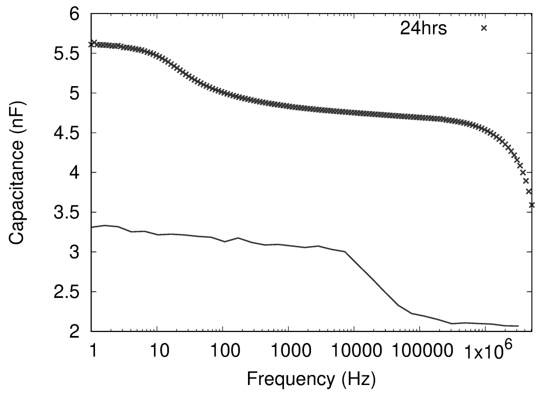


(e) Imaginary part of IS

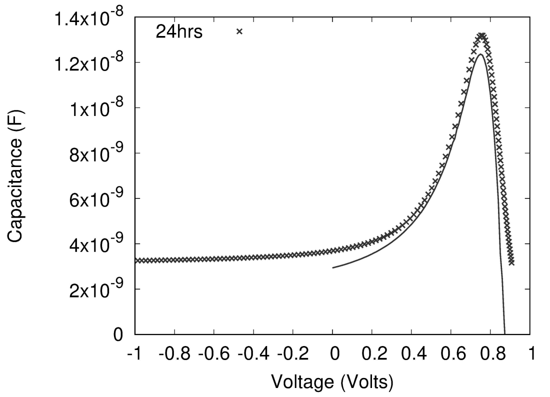


(f) Capacitance–Voltage

FIG. 17. Fits of the model to the 100 nm device at 24 h

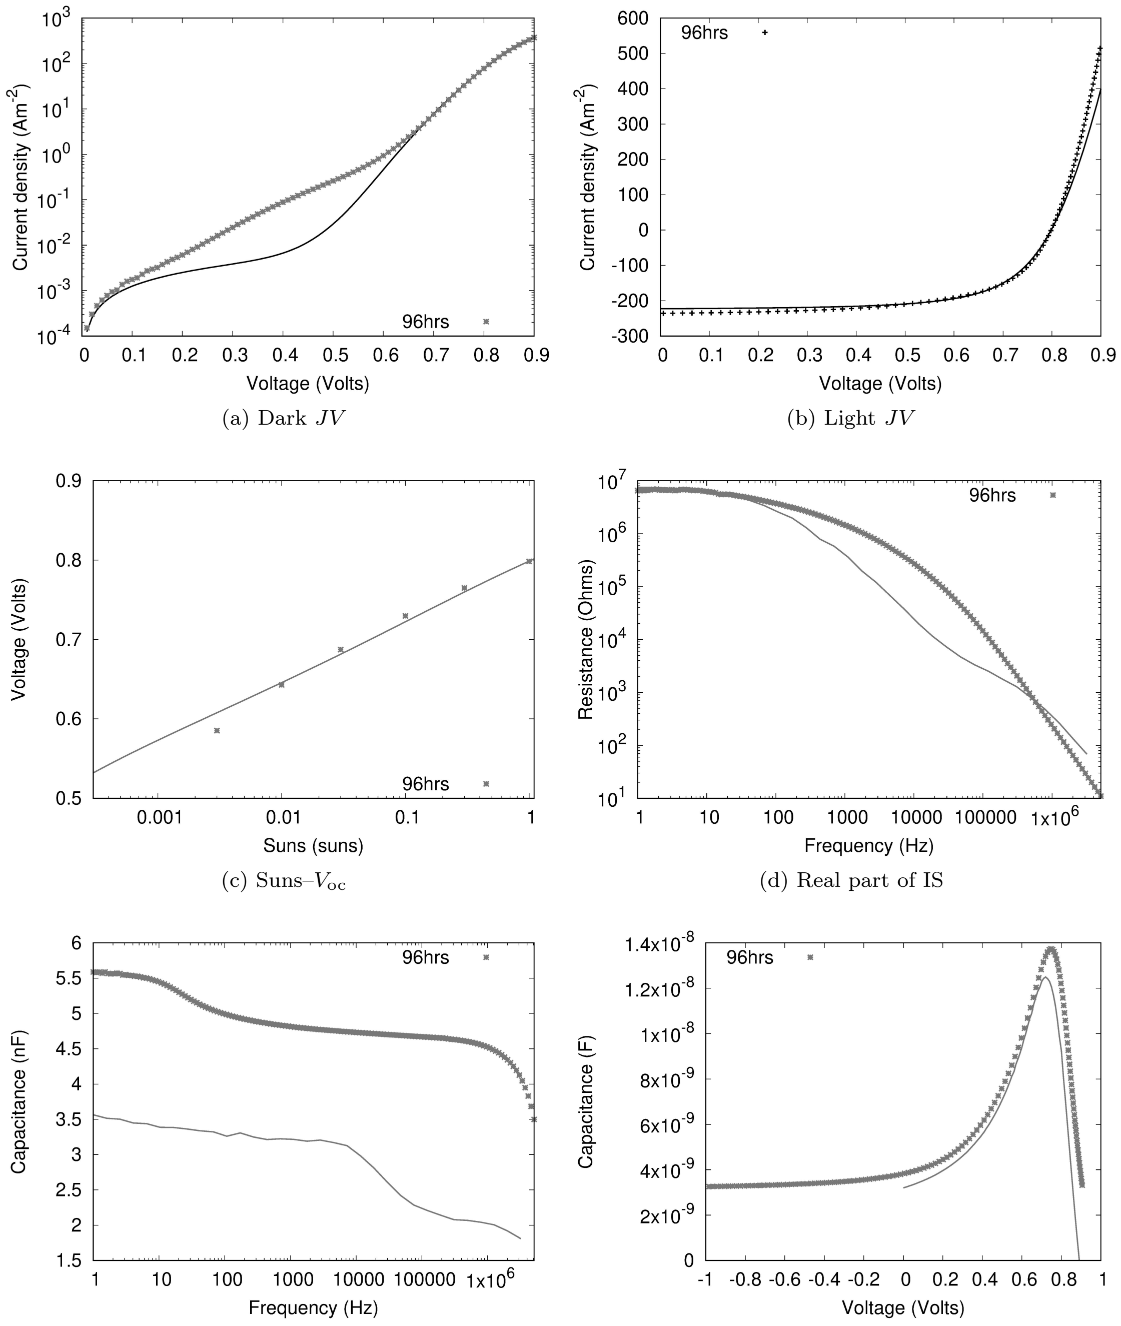


(a) Dark $JV$ (b) Light $JV$

(c) Suns–$V_{oc}$ (d) Real part of IS

(e) Imaginary part of IS (f) Capacitance–Voltage

FIG. 18. Fits of the model to the 100 nm device at 96 h

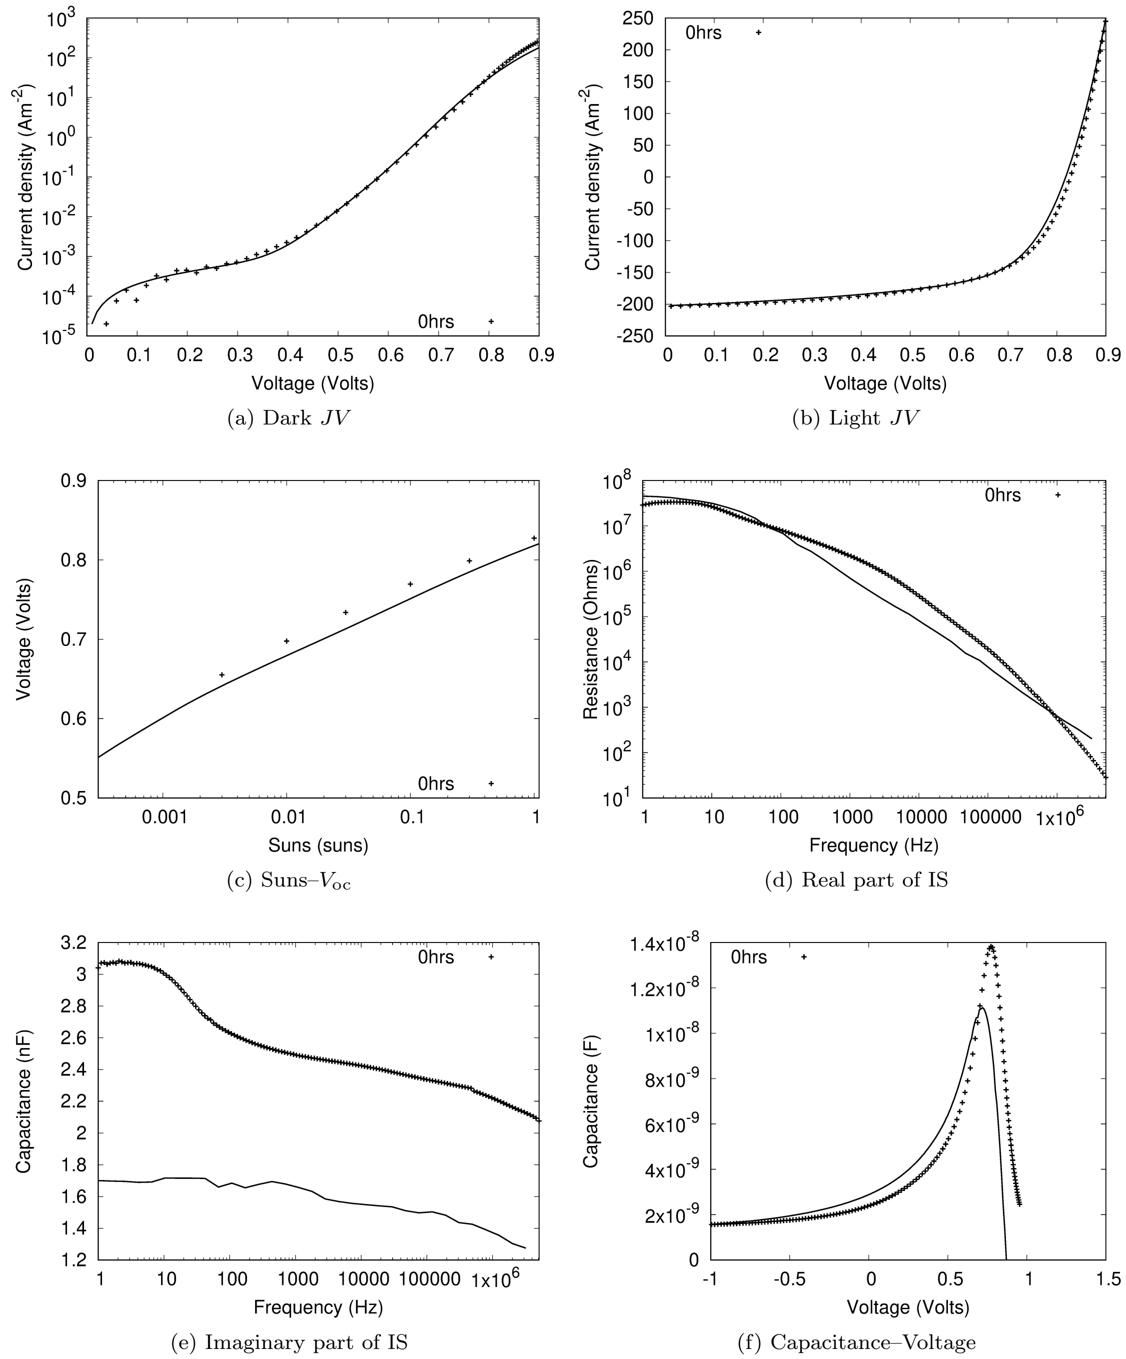


(a) Dark $JV$

(b) Light $JV$

(c) Suns–$V_{oc}$

(d) Real part of IS

(e) Imaginary part of IS

(f) Capacitance–Voltage

FIG. 19. Fits of the model to the 200 nm device at 0 h

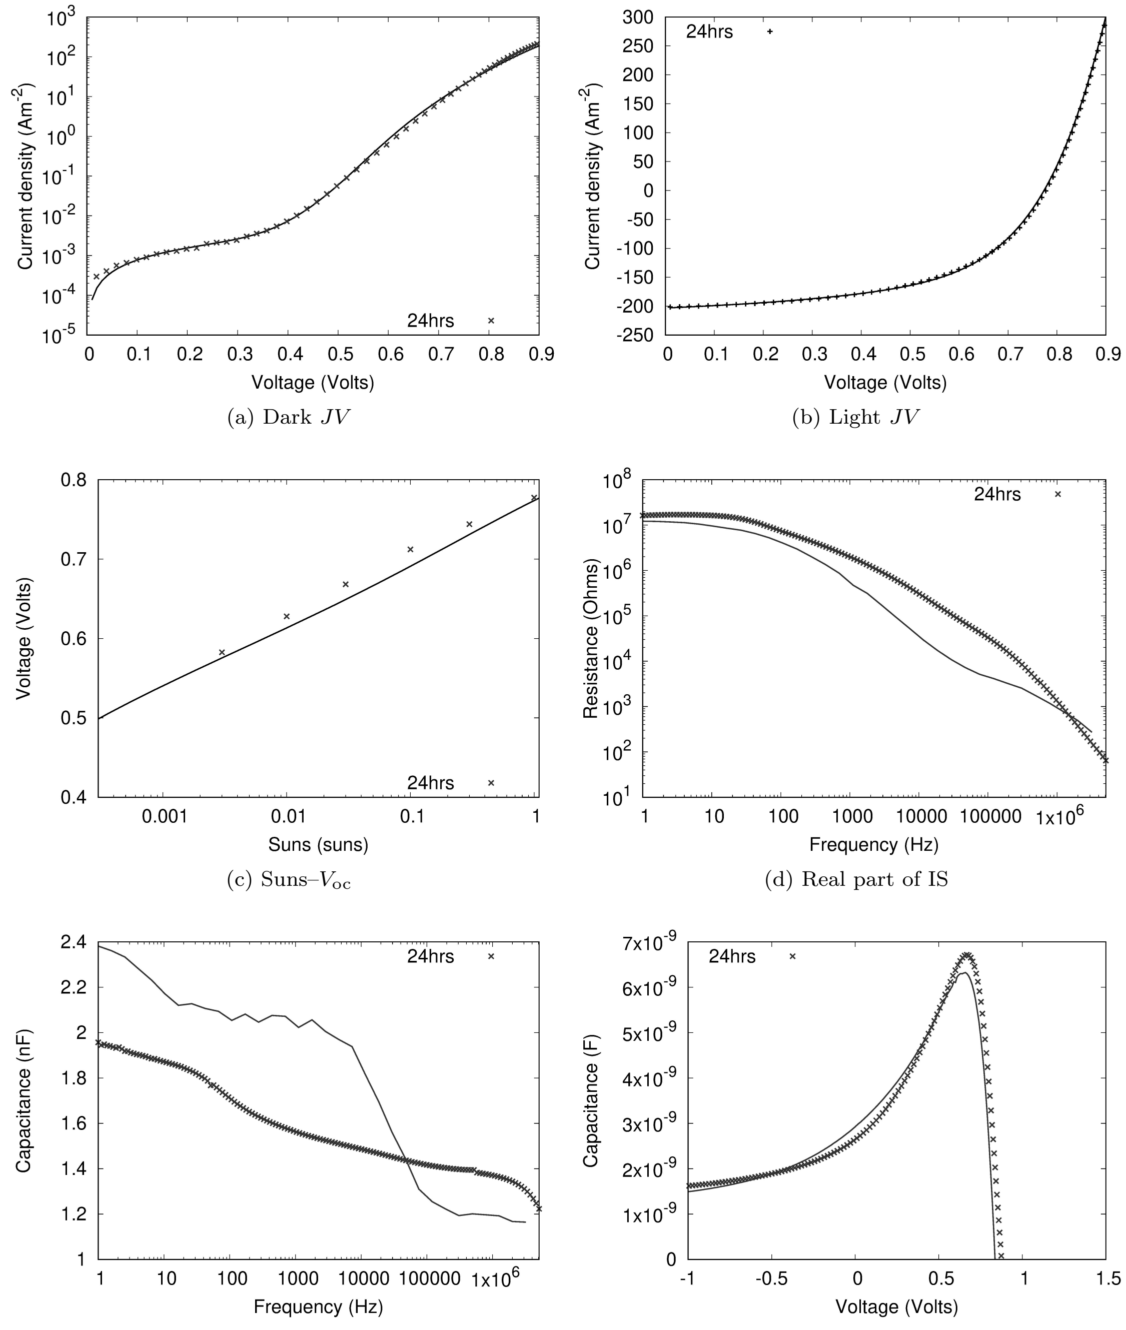


(a) Dark $JV$

(b) Light $JV$

(c) Suns–$V_{oc}$

(d) Real part of IS

(e) Imaginary part of IS

(f) Capacitance–Voltage

FIG. 20. Fits of the model to the 200 nm device at 24 h

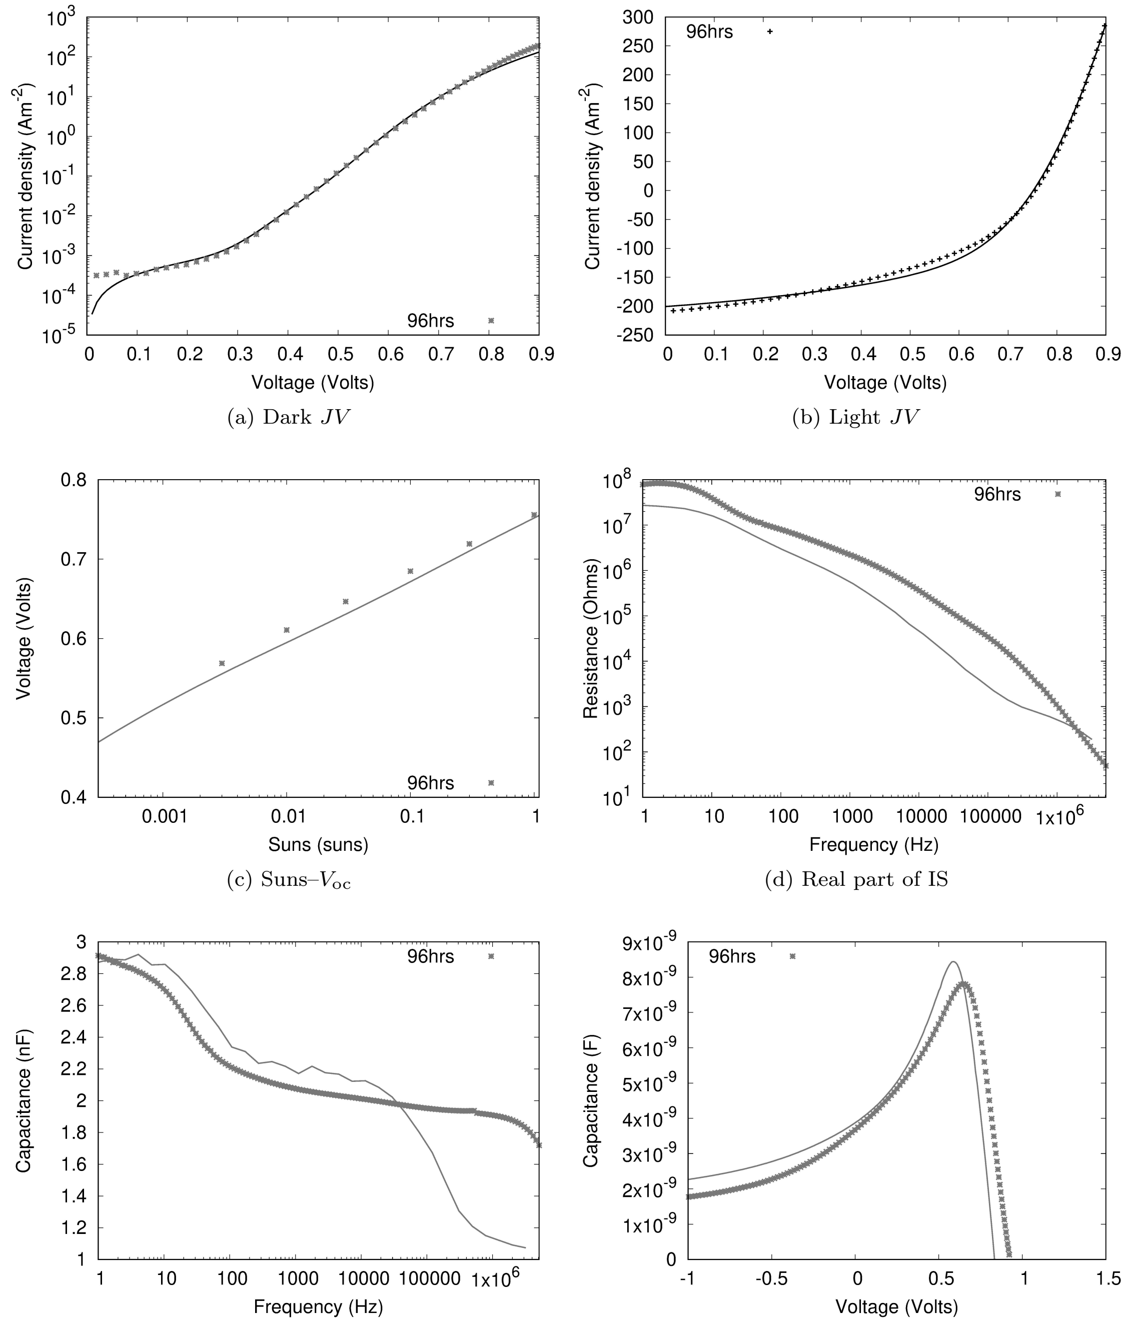


(a) Dark $JV$ (b) Light $JV$

(c) Suns–$V_{\rm oc}$ (d) Real part of IS

(e) Imaginary part of IS (f) Capacitance–Voltage

FIG. 21. Fits of the model to the 200 nm device at 96 h
